# Supplementary material for: AccuQuant: Simulating Multiple Denoising Steps for Quantizing Diffusion Models
Source: arXiv:2510.20348 source file (2025-10-23)
Supplement: Supplementary file 11 [file appendix_inference_computation.tex]

\begin{table}[!t]
    \centering
    \sisetup{detect-weight=true,detect-family=true,mode=text}
    \caption{Computational cost of real-time CPU inference. Experiments are conducted on CIFAR-10 ($32\times32$)~\cite{krizhevsky2009learning} with DDIM~\cite{song2020denoising} over 100 timesteps.}
    \label{tab:r6_cpu_cost}
    \vspace{5mm}
    
    \resizebox{1\textwidth}{!}{
    \begin{tabular}{l c c
                    S[table-format=4.0]
                    S[table-format=4.1]
                    S[table-format=3.3]
                    S[table-format=3.2]
                    S[table-format=1.2]}
        \toprule
        \textbf{Method} & \textbf{Bits (W/A)} & \textbf{Batch size}
        & {\textbf{GBops}}
        & {\textbf{Memory (MB)}}
        & {\textbf{CPU latency (s)}}
        & {\textbf{Model size (MB)}}
        & {\textbf{Speedup (×)}} \\
        \midrule
        Full-Precision           & 32/32 & 64 & 6597 & 1726.0 & 94.589 & 143.08 & 1.00 \\
        \midrule
        Q-Diffusion~\cite{li2023q}  & 8/8   & 64 &  798 & 1541.7 & 31.322 &  36.57 & 3.02 \\
        \cellcolor[HTML]{ECF9FF}Ours         & \cellcolor[HTML]{ECF9FF}8/8   & \cellcolor[HTML]{ECF9FF}64 &  \cellcolor[HTML]{ECF9FF}798 & \cellcolor[HTML]{ECF9FF}1541.7 & \cellcolor[HTML]{ECF9FF}31.380 &  \cellcolor[HTML]{ECF9FF}36.58 & \cellcolor[HTML]{ECF9FF}3.01 \\
        \bottomrule
    \end{tabular}}
\end{table}
